# Supplementary material for: Globally Continuous and Non-Markovian Activity Analysis from Videos
Source: arXiv:1810.04954 source file (2018-10-11)
Supplement: Supplementary file 2 [file supplement_cnaa.pdf]

# Supplementary Material of Globally Continuous and Non-Markovian Crowd Activity Analysis from Videos

He Wang<sup>1,2</sup> and Carol O’Sullivan<sup>1,3\*</sup>

<sup>1</sup> Disney Research Los Angeles\*\*, United States of America

<sup>2</sup> University of Leeds, United Kingdoms  
realcrane@gmail.com

<sup>3</sup> Trinity College Dublin, Ireland  
carol.osullivan@scss.tcd.ie

## 1 Generative Process of STHDP

We first again show the STHDP model in Figure 1.

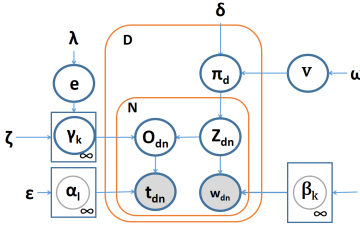

Fig. 1. STHDP model

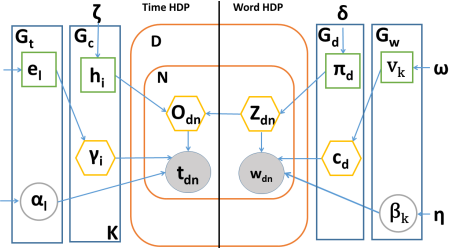

Fig. 2. Model used for sampling.

The generative process of Figure 1 is explained as follows:

1. Sample a corpus-level time base distribution,  $e|\lambda \sim GEM(\lambda)$
2. Sample a corpus-level word base distribution,  $v|\omega \sim GEM(\omega)$
3. For each corpus-level word topic  $k$ :
  - (a) Sample a distribution over words,  $\beta_k|\eta \sim Dirichlet(\eta)$
  - (b) Sample a word-topic-specific distribution over time topics,  $\gamma_k|e, \zeta \sim DP(\zeta, e)$
4. For each time topic  $l$ :
  - (a) Sample a distribution over time,  $\alpha_l|\Gamma \sim Normal-Inverse-Gamma(\Gamma)$
5. For each document  $d$ :
  - (a) Sample a distribution over topics,  $\pi_d|v, \sigma \sim DP(\sigma, v)$
  - (b) For each word  $n$ :
    - i. Sample a word topic indicator,  $z_{dn}|\pi_d \sim \pi_d$
    - ii. Sample a word  $w_{dn}|\beta_{z_{dn}} \sim Mult(\beta_{z_{dn}})$
    - iii. Sample a time topic indicator,  $o_{dn}|z_{dn}, \gamma \sim \gamma_{z_{dn}}$
    - iv. Sample a time word  $t_{dn}|\alpha_{o_{dn}} \sim Normal(\alpha_{o_{dn}})$

\* Correspondence Author

\*\* This work is mostly done by the authors when they were with Disney Research Los Angeles.

## 2 Gibbs Sampling for STHDP

Based on Figure 2, we only explain the modified Chinese Restaurant Franchise scheme here, as we fix the word HDP while running Chinese Restaurant Franchise (CRF) on the time HDP as in [1]. Following the naming convention in CRF, word topics and time topics are called **word dishes** and **time dishes**. Word documents are called **restaurants** and the set of time stamps associated with one word topic is called a **time restaurant**. A list of auxiliary variables are given in Table 1. Also, we use superscript to exclude data samples. For instance,  $z_j^{-ji}$  means the set of all table indicators in restaurant  $j$  excluding  $w_{ji}$ . Bold fonts means the whole set of some quartile, for instance, **I** means all time dish indices. We also use dots as summation.  $m_{\cdot k}$  is the number of word tables serving dish  $k$ .

**Table 1.** Variables in CRF

|              |                                                                        |
|--------------|------------------------------------------------------------------------|
| $v_w$        | a word in the vocabulary                                               |
| $V_w$        | the size of the vocabulary                                             |
| $w_{ji}$     | the $i$ th word in restaurant $j$                                      |
| $t_{ji}$     | the $i$ th time word in restaurant $j$                                 |
| $n_{ji}$     | the number of words in restaurant $j$ at table $i$                     |
| $n_{j\cdot}$ | the number of words in restaurant $j$                                  |
| $z_{ji}$     | the table indicator of the $i$ th word in restaurant $j$               |
| $k_{ji}$     | the dish indicator of the $i$ th word table in restaurant $j$          |
| $m_{jk}$     | the number of word tables in restaurant $j$ serving dish $k$           |
| $m_{j\cdot}$ | the number of word tables in restaurant $j$                            |
| $K$          | the number of word dishes                                              |
| $s_{ji}$     | the number of time words in time restaurant $j$ at time table $i$      |
| $s_{j\cdot}$ | the number of time words in time restaurant $j$                        |
| $d_{jl}$     | the number of time tables in time restaurant $j$ serving time dish $l$ |
| $d_{j\cdot}$ | the number of tables in time restaurant $j$                            |
| $o_{ji}$     | the table indicator of the $i$ th time word in time restaurant $j$     |
| $l_{ji}$     | the time dish indicator of the $i$ th table in time restaurant $j$     |

**Sampling Word Tables** The full conditional of a table indicator,  $z_{ji}$ , for a word,  $w_{ji}$ , given all other words is:

$$\begin{aligned}
 p(z_{ji} = z, w_{ji}, t_{ji} | \mathbf{z}^{-ji}, \mathbf{w}^{-ji}, \mathbf{t}^{-ji}, \mathbf{k}, \mathbf{o}^{-ji}, \mathbf{l}) = \\
 p(z_{ji} = z | \mathbf{z}^{-ji}) \\
 p(w_{ji} | t_{ji}, z_{ji} = z, k_{jz} = k, \mathbf{w}^{-ji}, \mathbf{z}^{-ji}, \mathbf{k}, \mathbf{t}^{-ji}, \mathbf{o}^{-ji}, \mathbf{l}) \\
 p(t_{ji} | z_{ji} = z, k_{jz} = k, \mathbf{t}^{-ji}, \mathbf{o}^{-ji}, \mathbf{l})
 \end{aligned} \tag{1}$$

where

$$p(z_{ji} = z | \mathbf{z}^{-ji}) \propto \begin{cases} n_{jz} & \text{if } z \text{ is an existing table} \\ \delta & \text{otherwise} \end{cases} \quad (2)$$

$$\begin{aligned} p(w_{ji} | t_{ji}, z_{ji} = z, k_{jz} = k, \mathbf{w}^{-ji}, \mathbf{z}^{-ji}, \mathbf{k}, \mathbf{t}^{-ji}, \mathbf{o}^{-ji}, \mathbf{l}) \\ \propto \begin{cases} f_{k_z}(w_{ji}) & \text{if } z \text{ exists} \\ m_{\cdot k} f_k(w_{ji}) & \text{else if } k \text{ exists} \\ \omega f_{k_{new}}(w_{ji}) & \text{otherwise} \end{cases} \end{aligned} \quad (3)$$

where  $f$  is the conditional density of  $w_{ji}$  given all other variables.  $p(t_{ji} | z_{ji} = z, k_{jz} = k, \mathbf{t}^{-ji}, \mathbf{o}^{-ji}, \mathbf{l})$  is the extra term from the time HDP that needs special treatment. If, for every word, we do sampling conditioned on its time word in the time HDP, it is very slow. So we marginalize over all time tables in the time restaurant.

$$\begin{aligned} p(t_{ji} | z_{ji} = z, k_{jz} = k, \mathbf{t}^{-ji}, \mathbf{o}^{-ji}, \mathbf{l}) = \\ \sum_{o=1}^{d_j} p(o_{ji} = o | z_{ji} = z, k_{jz} = k, \mathbf{t}^{-ji}, \mathbf{o}^{-ji}) \\ p(t_{ji} | o_{ji} = o, l_{jo} = l, \mathbf{l}) \end{aligned} \quad (4)$$

$$\begin{aligned} p(o_{ji} = o | z_{ji} = z, k_{jz} = k, \mathbf{t}^{-ji}, \mathbf{o}^{-ji}) \\ \propto \begin{cases} s_{ji} & \text{if } o \text{ exists} \\ \zeta & \text{otherwise} \end{cases} \end{aligned} \quad (5)$$

$$p(t_{ji} | o_{ji} = o, l_{jo_{ji}} = l, \mathbf{l}) \propto \begin{cases} g_{l_o}(t_{ji}) & \text{if } o \text{ exists} \\ d_{\cdot l} g_l(t_{ji}) & \text{else if } l \text{ exists} \\ \varepsilon g_{l_{new}}(t_{ji}) & \text{otherwise} \end{cases} \quad (6)$$

where  $g$  is the posterior predictive distribution of a Gaussian, a t-Distribution.

**Sampling Word Dishes** Sampling a word topic for a word table  $z$  in restaurant  $j$ , with the associated words  $\mathbf{w}_{jz}$  and time words  $\mathbf{t}_{jz}$ , follows:

$$\begin{aligned} p(k_{jz} = k, \mathbf{w}_{jz}, \mathbf{t}_{jz} | \mathbf{w}^{-jz}, \\ \mathbf{t}^{-jz}, \mathbf{z}^{-jz}, \mathbf{k}^{-jz}, \mathbf{o}^{-jz}, \mathbf{l}^{-jz}) \\ \propto \begin{cases} m_{\cdot k}^{-jz} p(\mathbf{w}_{jz} | \bullet) p(\mathbf{t}_{jz} | \bullet) & \text{if } k \text{ exists} \\ \omega p(\mathbf{w}_{jz} | \bullet) p(\mathbf{t}_{jz} | \bullet) & \text{otherwise} \end{cases} \end{aligned} \quad (7)$$

where  $\bullet$  means all the other variables the distribution is conditioned on.  $p(\mathbf{w}_{jz} | \bullet) = f_k(\mathbf{w}_{jz})$ . To fully compute  $p(\mathbf{t}_{jz} | \bullet) = p(\mathbf{t}_{jz} | k_z = k, \mathbf{o}^{-jz}, \mathbf{l}^{-jz})$  is too expensive because table  $z$  might have many words. So we randomly sample a number of them to compute  $\hat{p}(\mathbf{t}_{jz} | \bullet)$  as an approximation, which can be computed by Equation 4.

### 3 Additional Results

We show some additional patterns in the Forum dataset and TrainStation dataset in Figure 3 and Figure 4.

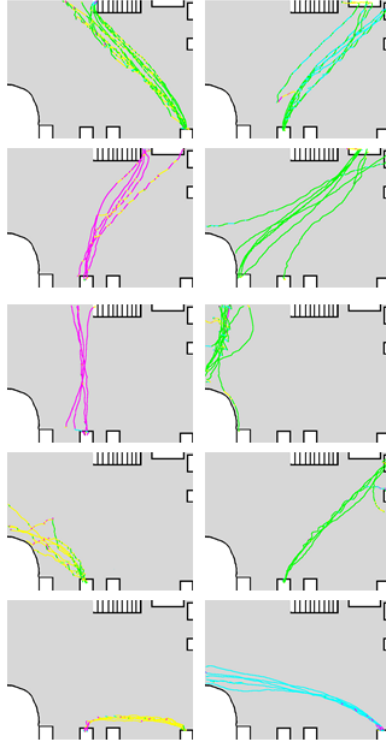

**Fig. 3.** Additional Patterns in Forum dataset

### References

1. Teh, Y.W., Jordan, M.I., Beal, M.J., Blei, D.M.: Hierarchical Dirichlet Processes. J. Am. Stat. Assoc. **101**(476) (2006) 1566–1581

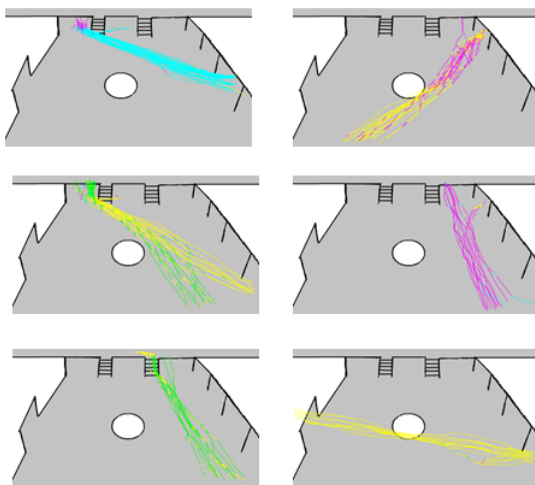

**Fig. 4.** Additional Patterns in TrainStationAdditional dataset
